# Supplementary material for: Recursive-Head Geometry and Order-Free Efficient Inference in Finite-State Nested Markov Models
Source: arXiv:2609.17939 source file (2026-09-15)
Supplement: Supplementary file 1 [file external_labels_main.tex]

%% GENERATED from the other document's .aux by tools/make_label_tables.py; do not edit.
\externallabel{app:B-cyclic}{B.2}{43}
\externallabel{app:B-finite-sample}{B.9}{56}
\externallabel{app:B-intervention}{B.5}{48}
\externallabel{app:B-mixed}{B.4}{47}
\externallabel{app:B-mixture}{B.11}{58}
\externallabel{app:B-primary}{B.1}{40}
\externallabel{app:B-repro}{B.8}{53}
\externallabel{app:B-sequential}{B.7}{50}
\externallabel{app:B-shortcuts}{B.10}{57}
\externallabel{app:B-targeting}{B.6}{49}
\externallabel{app:B-three}{B.3}{45}
\externallabel{app:er-rrs-compatibility}{A.3.3}{10}
\externallabel{app:finite-state-parameterization-proof}{A.3}{6}
\externallabel{app:notation}{A.2}{3}
\externallabel{app:proofs}{A.4}{17}
\externallabel{app:proofs-bridge}{A.4.4}{23}
\externallabel{app:proofs-counterexample}{A.4.3}{22}
\externallabel{app:proofs-geometry}{A.4.2}{19}
\externallabel{app:proofs-sequential}{A.4.6}{34}
\externallabel{app:proofs-setup}{A.4.1}{18}
\externallabel{app:proofs-targeted}{A.4.5}{28}
\externallabel{app:prototype-ledger}{B}{40}
\externallabel{app:results-scope}{A.1}{2}
\externallabel{eq:BY-attribution-ratio}{B.4}{42}
\externallabel{eq:BY-constraint-map}{B.3}{42}
\externallabel{eq:appendix-algebraic-district-split}{A.2}{7}
\externallabel{eq:appendix-ancestral-peeling}{A.3}{7}
\externallabel{eq:appendix-corner-reconstruction}{A.6}{9}
\externallabel{eq:appendix-rf-margin}{A.1}{6}
\externallabel{eq:appendix-top-head-coordinate}{A.4}{9}
\externallabel{eq:appendix-top-head-partition}{A.5}{9}
\externallabel{eq:cyclic-counterexample-graph}{B.5}{43}
\externallabel{eq:cyclic-cross-district-gram-zero}{B.6}{43}
\externallabel{eq:cyclic-rational-coordinates}{B.9}{44}
\externallabel{eq:cyclic-raw-direction-failure}{B.8}{43}
\externallabel{eq:cyclic-raw-directions}{B.7}{43}
\externallabel{eq:district-fixing-composition}{A.9}{21}
\externallabel{eq:interleaved-source-nuisance-fixture}{B.17}{51}
\externallabel{eq:interleaved-source-rational-sem}{B.16}{50}
\externallabel{eq:inverse-identities}{A.7}{19}
\externallabel{eq:left-inverse-differential}{A.8}{19}
\externallabel{eq:observational-block-is-native-factor}{A.11}{36}
\externallabel{eq:three-district-control-graph}{B.10}{45}
\externallabel{eq:three-district-pairwise-orthogonality}{B.12}{46}
\externallabel{eq:three-district-projection-residuals}{B.13}{46}
\externallabel{eq:three-district-rational-coordinates}{B.15}{47}
\externallabel{eq:three-district-raw-residuals}{B.11}{46}
\externallabel{eq:three-district-third-moment}{B.14}{46}
\externallabel{eq:two-transition-both-wrong-fixture}{B.20}{51}
\externallabel{eq:two-transition-control-fixtures}{B.21}{52}
\externallabel{eq:two-transition-rational-sem}{B.18}{51}
\externallabel{eq:two-transition-true-nuisances}{B.19}{51}
\externallabel{eq:uniform-targeting-slope}{A.10}{33}
\externallabel{eq:verma-active-latent-sem}{B.2}{42}
\externallabel{eq:verma-rational-sem}{B.1}{41}
\externallabel{eq:verma-variant-rational-sem}{B.22}{53}
\externallabel{eq:verma-variant-values}{B.23}{53}
\externallabel{fig:cyclic-counterexample-graph}{S1}{43}
\externallabel{fig:three-district-control-graph}{S2}{46}
\externallabel{lem:intrinsic-set-bridge}{A.2}{11}
\externallabel{lem:rf-implies-markov}{A.3}{12}
\externallabel{lem:signed-factor-positivity}{A.1}{7}
\externallabel{prop:er-rrs-compatibility-full}{A.4}{12}
\externallabel{tab:finite-sample-variance-comparison}{S3}{57}
\externallabel{tab:results-scope-summary}{S1}{2}
\externallabel{tab:verma-exact-computational-checks}{S2}{43}
