# Supplementary material for: Recursive-Head Geometry and Order-Free Efficient Inference in Finite-State Nested Markov Models
Source: arXiv:2609.17939 source file (2026-09-15)
Supplement: Supplementary file 2 [file external_labels_supplement.tex]

%% GENERATED from the other document's .aux by tools/make_label_tables.py; do not edit.
\externallabel{ass:mr-sequential-transport}{7.2}{36}
\externallabel{cor:active-factor-locality}{5.4}{20}
\externallabel{cor:active-side-nested-geometry}{5.6}{21}
\externallabel{cor:block-directness}{3.3}{12}
\externallabel{cor:exact-empirical-eif-equation}{6.15}{31}
\externallabel{cor:excluded-source-native-block}{5.9}{22}
\externallabel{cor:exogenous-source-mixture}{5.13}{24}
\externallabel{cor:explicit-eif}{6.1}{25}
\externallabel{cor:fisher-chart-pullback}{3.2}{12}
\externallabel{cor:same-sample-one-step}{6.10}{29}
\externallabel{cor:source-slice-foldwise-unbiased}{6.8}{28}
\externallabel{cor:source-standardized-complementary-blocks}{5.16}{24}
\externallabel{cor:source-standardized-eif}{5.14}{24}
\externallabel{cor:tmle-substitution}{6.17}{32}
\externallabel{def:admissible-source-law}{5.10}{22}
\externallabel{eq:active-ancestral-set}{5.1}{18}
\externallabel{eq:active-chart-bridge}{5.8}{21}
\externallabel{eq:active-chart-domain}{5.9}{21}
\externallabel{eq:active-chart-score}{5.11}{21}
\externallabel{eq:active-chart-score-operator}{5.10}{21}
\externallabel{eq:active-factor-score-sum}{5.12}{21}
\externallabel{eq:active-intrinsicness}{5.2}{18}
\externallabel{eq:active-tail-restriction}{5.4}{20}
\externallabel{eq:admissible-candidate-weight}{7.10}{38}
\externallabel{eq:algebraic-normalization}{2.6}{9}
\externallabel{eq:cadmg-coordinate-extraction}{2.7}{9}
\externallabel{eq:cadmg-positive-coordinate-domain}{2.9}{10}
\externallabel{eq:coherent-eif-map}{6.2}{26}
\externallabel{eq:coherent-second-order-remainder}{6.6}{27}
\externallabel{eq:configured-factor-reassembly}{5.6}{20}
\externallabel{eq:coordinate-extraction}{2.3}{7}
\externallabel{eq:corrected-ladder-normalization}{7.6}{37}
\externallabel{eq:cross-fitted-exact-expansion}{6.12}{28}
\externallabel{eq:cross-fitted-one-step}{6.11}{28}
\externallabel{eq:direct-intervention-eif}{5.15}{22}
\externallabel{eq:district-domain-product}{3.6}{13}
\externallabel{eq:district-factor-as-fixing}{3.7}{13}
\externallabel{eq:district-gram-projection}{3.8}{14}
\externallabel{eq:district-space}{3.3}{12}
\externallabel{eq:eif-projection}{6.1}{24}
\externallabel{eq:exact-empirical-eif-equation}{6.23}{31}
\externallabel{eq:exact-one-step-remainder}{6.7}{27}
\externallabel{eq:exact-sequential-drift}{7.12}{38}
\externallabel{eq:exact-source-block-cancellation}{6.9}{27}
\externallabel{eq:finite-direction-rectangle}{3.1}{11}
\externallabel{eq:fisher-chart-matrix}{3.2}{12}
\externallabel{eq:fixing-kernel-bridge}{2.1}{7}
\externallabel{eq:full-history-propensity-ladder}{7.4}{37}
\externallabel{eq:general-coordinate-block}{2.2}{7}
\externallabel{eq:general-forward-map}{2.4}{8}
\externallabel{eq:global-gram-projection}{3.9}{14}
\externallabel{eq:imported-intervention-product}{5.3}{19}
\externallabel{eq:independent-source-mixture-and-mean}{5.16}{23}
\externallabel{eq:independent-source-mixture-derivative}{5.18}{23}
\externallabel{eq:independent-source-mixture-eif}{5.19}{23}
\externallabel{eq:intervention-chart-derivative}{5.13}{22}
\externallabel{eq:intervention-coordinate-derivative}{5.14}{22}
\externallabel{eq:least-favorable-chart-ode}{6.21}{31}
\externallabel{eq:least-favorable-score-identity}{6.22}{31}
\externallabel{eq:local-eif-stability-bounds}{6.3}{26}
\externallabel{eq:mixture-coordinate-contributions}{5.17}{23}
\externallabel{eq:mixture-error-decompositions}{6.4}{27}
\externallabel{eq:modular-coefficient-identity}{6.17}{30}
\externallabel{eq:modular-eif-extra-remainder}{6.18}{30}
\externallabel{eq:modular-eif-rate}{6.19}{30}
\externallabel{eq:mr-block-partition}{7.3}{36}
\externallabel{eq:mr-sequential-kernel-interface}{7.5}{37}
\externallabel{eq:one-step-asymptotic-linearity}{6.13}{28}
\externallabel{eq:one-step-initial-rate}{6.10}{28}
\externallabel{eq:quadratic-one-step-bound}{6.8}{27}
\externallabel{eq:reachable-chart-realization}{3.5}{13}
\externallabel{eq:robust-transition-centering}{7.11}{38}
\externallabel{eq:sequential-asymptotic-linearity}{7.17}{39}
\externallabel{eq:sequential-canonical-projection}{7.18}{40}
\externallabel{eq:sequential-consistency-product}{7.15}{39}
\externallabel{eq:sequential-cross-fitted-estimator}{7.13}{38}
\externallabel{eq:sequential-influence-function}{7.16}{39}
\externallabel{eq:sequential-outcome-recursion}{7.9}{38}
\externallabel{eq:sequential-prefix-bridge}{7.7}{37}
\externallabel{eq:sequential-prefix-transport}{7.8}{38}
\externallabel{eq:sequential-pythagoras}{7.19}{40}
\externallabel{eq:smooth-mixture-second-derivative}{6.5}{27}
\externallabel{eq:source-isolation}{7.1}{36}
\externallabel{eq:source-slice-cross-fitted-representation}{6.15}{29}
\externallabel{eq:source-slice-foldwise-unbiasedness}{6.14}{29}
\externallabel{eq:source-slice-mean-square-rate}{6.16}{29}
\externallabel{eq:source-standardization-law}{5.20}{24}
\externallabel{eq:source-standardized-eif}{5.22}{24}
\externallabel{eq:source-standardized-weight-coordinate}{5.21}{24}
\externallabel{eq:source-tail-coverage}{7.2}{36}
\externallabel{eq:standing-import-inverses}{2.8}{10}
\externallabel{eq:statistical-intervention-functional}{5.7}{21}
\externallabel{eq:sterile-marginalization}{2.5}{9}
\externallabel{eq:tail-slice-map}{5.5}{20}
\externallabel{eq:targeting-coordinate-field}{6.20}{30}
\externallabel{eq:tmle-asymptotic-linearity}{6.26}{32}
\externallabel{eq:tmle-one-step-equivalence}{6.27}{32}
\externallabel{eq:tmle-root-rate}{6.24}{31}
\externallabel{eq:tmle-updated-rate}{6.25}{32}
\externallabel{eq:top-level-factorization}{3.4}{12}
\externallabel{eq:transition-union-regime}{7.14}{38}
\externallabel{eq:verma-counterexample-graph}{4.1}{15}
\externallabel{eq:verma-district-codimension-seven}{4.4}{17}
\externallabel{eq:verma-district-score-containment}{4.3}{16}
\externallabel{eq:verma-normalized-district-score-space}{4.2}{16}
\externallabel{ex:split-boundary-nonidentification}{5.2}{20}
\externallabel{ex:tmle-source-slice-failure}{6.21}{33}
\externallabel{fig:verma-counterexample-graph}{1}{15}
\externallabel{lem:algebraic-district-factorization}{3.4}{12}
\externallabel{lem:algebraic-normalization}{2.4}{9}
\externallabel{lem:configured-factor-reassembly}{5.3}{20}
\externallabel{lem:exact-one-step-remainder}{6.4}{27}
\externallabel{lem:mixture-error-bookkeeping}{6.3}{26}
\externallabel{lem:reachable-chart-realization}{3.5}{13}
\externallabel{lem:sequential-transport-centering}{7.4}{38}
\externallabel{lem:source-isolated-active-block-slice}{7.3}{37}
\externallabel{lem:sterile-marginalization}{2.3}{9}
\externallabel{prop:causal-identification-interface}{5.1}{19}
\externallabel{prop:district-locality}{3.6}{13}
\externallabel{prop:er-equivalence-rrs-compatibility}{2.1}{6}
\externallabel{prop:estimated-eif-stability}{6.2}{26}
\externallabel{prop:gram-projection}{3.10}{14}
\externallabel{prop:modular-eif-remainder}{6.12}{29}
\externallabel{prop:mr-block-order-screen}{7.1}{36}
\externallabel{prop:positive-smooth-source-mixture}{5.11}{23}
\externallabel{prop:raw-failure}{4.1}{16}
\externallabel{prop:sequential-strict-variance-gap}{7.8}{40}
\externallabel{prop:source-block-drift-cancellation}{6.5}{27}
\externallabel{prop:standing-finite-state-import}{2.5}{9}
\externallabel{prop:targeting-coordinate-lift}{6.13}{30}
\externallabel{rem:chart-not-projection}{3.11}{14}
\externallabel{rem:cyclic-quotient-diagnostic}{3.9}{14}
\externallabel{rem:forward-map-multiaffine}{2.2}{9}
\externallabel{rem:independent-not-natural-source}{5.15}{24}
\externallabel{rem:p-dependent-source-law}{5.17}{24}
\externallabel{rem:robustness-count-comparison}{7.9}{41}
\externallabel{rem:statistical-not-causal-extension}{5.7}{21}
\externallabel{rem:straight-line-numerical-targeting}{6.19}{32}
\externallabel{rem:verma-variant}{7.10}{42}
\externallabel{sec:counterexample}{4}{15}
\externallabel{sec:cyclic-control}{4.4}{17}
\externallabel{sec:discussion}{9}{43}
\externallabel{sec:finite-sample}{8}{42}
\externallabel{sec:geometry}{3}{11}
\externallabel{sec:intervention-bridge}{5}{17}
\externallabel{sec:introduction}{1}{2}
\externallabel{sec:sequential-union}{7}{35}
\externallabel{sec:setup}{2}{4}
\externallabel{sec:shortcuts}{7.1}{35}
\externallabel{sec:targeted}{6}{24}
\externallabel{sec:three-district-raw-control}{4.5}{17}
\externallabel{subsec:one-step-tmle-contrast}{6.4}{33}
\externallabel{tab:efficient-sequential-comparison}{2}{41}
\externallabel{tab:one-step-tmle-contrast}{1}{34}
\externallabel{thm:chart-tmle}{6.16}{31}
\externallabel{thm:coherent-one-step}{6.7}{28}
\externallabel{thm:district-orthogonality}{3.8}{13}
\externallabel{thm:exact-sequential-drift}{7.5}{38}
\externallabel{thm:forward-chart}{3.1}{11}
\externallabel{thm:independent-source-mixture-eif}{5.12}{23}
\externallabel{thm:intervention-chart-eif}{5.8}{22}
\externallabel{thm:least-favorable-chart-flow}{6.14}{31}
\externallabel{thm:normalized-intervention-bridge}{5.5}{21}
\externallabel{thm:sequential-multiple-robustness}{7.6}{39}
\externallabel{thm:sequential-projection-comparison}{7.7}{40}
