# Supplementary material for: Recursive-Head Geometry and Order-Free Efficient Inference in Finite-State Nested Markov Models
Source: arXiv:2609.17939 source file (2026-09-15)
Supplement: Supplementary file 3 [file preamble_shared.tex]

%% Shared preamble of the main paper and the Supplementary Material (P2 packaging candidate, 2026-09-12).
%% The packages and local definitions are the accepted main.tex preamble, moved verbatim; the \externallabel
%% macro below is the only addition.

%% Packages
\RequirePackage{amsthm,amsmath,amsfonts,amssymb}
\RequirePackage{array,booktabs,enumitem,float}
\RequirePackage{longtable}%% supplement notation index
\RequirePackage{needspace}%% keep a section heading with its opening text (Section 9)
%% Section 4 and Appendix B graph figures.
\RequirePackage{tikz}
\usetikzlibrary{arrows.meta}
\RequirePackage[numbers]{natbib}

%\RequirePackage[authoryear]{natbib}%% uncomment this for author-year citations
\RequirePackage[colorlinks,citecolor=blue,urlcolor=blue]{hyperref}
\RequirePackage{graphicx}%% \scalebox for \bigtimes

\startlocaldefs
%%%%%%%%%%%%%%%%%%%%%%%%%%%%%%%%%%%%%%%%%%%%%%
%%                                          %%
%% Uncomment next line to change            %%
%% the type of equation numbering           %%
%%                                          %%
%%%%%%%%%%%%%%%%%%%%%%%%%%%%%%%%%%%%%%%%%%%%%%
\numberwithin{equation}{section}
%%%%%%%%%%%%%%%%%%%%%%%%%%%%%%%%%%%%%%%%%%%%%%
%%                                          %%
%% For Axiom, Claim, Corollary, Hypothesis, %%
%% Lemma, Theorem, Proposition              %%
%% use \theoremstyle{plain}                 %%
%%                                          %%
%%%%%%%%%%%%%%%%%%%%%%%%%%%%%%%%%%%%%%%%%%%%%%
%\theoremstyle{plain}
%\newtheorem{???}{???}
%\newtheorem*{???}{???}
%\newtheorem{???}{???}[???]
%\newtheorem{???}[???]{???}
%%%%%%%%%%%%%%%%%%%%%%%%%%%%%%%%%%%%%%%%%%%%%%
%%                                          %%
%% For Assumption, Definition, Example,     %%
%% Notation, Property, Remark, Fact         %%
%% use \theoremstyle{definition}            %%
%%                                          %%
%%%%%%%%%%%%%%%%%%%%%%%%%%%%%%%%%%%%%%%%%%%%%%
%\theoremstyle{definition}
%\newtheorem{???}{???}
%\newtheorem*{???}{???}
%\newtheorem{???}{???}[???]
%\newtheorem{???}[???]{???}
%%%%%%%%%%%%%%%%%%%%%%%%%%%%%%%%%%%%%%%%%%%%%%
%% Please put your definitions here:        %%
\newtheorem{theorem}{Theorem}[section]
\newtheorem{lemma}[theorem]{Lemma}
\newtheorem{proposition}[theorem]{Proposition}
\newtheorem{corollary}[theorem]{Corollary}
\theoremstyle{definition}
\newtheorem{definition}[theorem]{Definition}
\newtheorem{assumption}[theorem]{Assumption}
\newtheorem{example}[theorem]{Example}
% \theoremstyle{remark}
\newtheorem{remark}[theorem]{Remark}

\newcommand{\cG}{\mathcal G}
\newcommand{\cN}{\mathcal N}
\newcommand{\cD}{\mathcal D}
\newcommand{\cI}{\mathcal I}
\newcommand{\cS}{\mathcal S}
\newcommand{\cT}{\mathcal T}
\newcommand{\cX}{\mathfrak X}
\newcommand{\R}{\mathbb R}
\newcommand{\E}{\mathrm E}
\newcommand{\pr}{\mathrm P}
\newcommand{\pa}{\operatorname{pa}}
\newcommand{\dis}{\operatorname{dis}}
\newcommand{\ran}{\operatorname{ran}}
\newcommand{\Span}{\operatorname{span}}
\newcommand{\proj}{\operatorname{proj}}
\newcommand{\EIF}{\operatorname{EIF}}
\newcommand{\ind}{\mathrel{\perp\!\!\!\perp}}
\newcommand{\given}{\,\middle|\,}
%% Cartesian-product operator (the only symbol formerly taken from mathabx):
%% a scaled \times, sized by math style, with limits placed as for \prod.
\newcommand{\bigtimes}{\mathop{\mathchoice{\vcenter{\hbox{\scalebox{1.7}{$\times$}}}}{\vcenter{\hbox{\scalebox{1.25}{$\times$}}}}{\vcenter{\hbox{\scalebox{0.9}{$\times$}}}}{\vcenter{\hbox{\scalebox{0.7}{$\times$}}}}}\displaylimits}
%%%%%%%%%%%%%%%%%%%%%%%%%%%%%%%%%%%%%%%%%%%%%%

\endlocaldefs

%% Cross-document references: the imsart class forbids the xr/xr-hyper packages ('External references are not
%% supported in our workflow. Replace all references to external documents with plain text.'), so the numbers of
%% the other document's labels are supplied as plain text by a GENERATED table
%% (sections/supplement/external_labels_<document>.tex, produced from the other document's aux by
%% tools/p2_build_measure.py) of \externallabel{label}{number}{page} definitions; \ref/\eqref then typeset the
%% number without a hyperlink (hyperref suppresses the link with an empty target, one notice per use).
\makeatletter
\newcommand{\externallabel}[3]{\expandafter\gdef\csname r@#1\endcsname{{#2}{#3}{}{}{}}}
\makeatother

%% The arXiv version of this article is a single document that ships without the reproducibility-artifact
%% archive, so Appendix B.8 summarises that archive there instead of listing its contents (advisor and CP
%% decision, 13 September 2026).  The switch is FALSE here: the journal article and supplement select the
%% accepted text, and only the generated arXiv root (main_arxiv.tex) sets it true.  No accepted prose is
%% removed -- the full list is the \else branch of one conditional in B_prototype_ledger.tex.
\newif\ifarxivversion
\arxivversionfalse
